# Supplementary material for: Sequential Semantic-Non-Semantic Watermarking: Robustness Against UnMarker Attacks
Source: arXiv:2611.20115 source file (2026-11-15)
Supplement: Supplementary file 1 [file detailed_experimental_results.tex]

\section{Appendix - Detailed experimental results} \label{chap: Detailed Experimental Results}
\subsection{Phase 1: Baseline study}
\begingroup
\small
\setlength{\tabcolsep}{4pt}
\renewcommand{\arraystretch}{0.95}

\begin{longtable}{lcccc}
\caption{Base HiDDeN attacked by \textbf{non-semantic attack}: per-image bit accuracy before watermarking ($\mathrm{BA}_{\text{orig}}$), after watermarking ($\mathrm{BA}_{\text{wm}}$), and after removal ($\mathrm{BA}_{\text{att}}$), with similarity score. Images 1--25: COCO, 26--50: CelebA.}
\label{tab:hidden_base_nonsemantic}\\
\toprule
Image & $\mathrm{BA}_{\text{orig}}$ & $\mathrm{BA}_{\text{wm}}$ & $\mathrm{BA}_{\text{att}}$ & Similarity Score \\
\midrule
\endfirsthead

\toprule
Image & $\mathrm{BA}_{\text{orig}}$ & $\mathrm{BA}_{\text{wm}}$ & $\mathrm{BA}_{\text{att}}$ & Similarity Score \\
\midrule
\endhead

\midrule
\multicolumn{5}{r}{\textit{Continued on next page}}\\
\endfoot

\bottomrule
\endlastfoot

image\_1  & 0.630 & 1.000 & 0.600 & 0.065 \\
image\_2  & 0.570 & 1.000 & 0.470 & 0.092 \\
image\_3  & 0.500 & 1.000 & 0.500 & 0.074 \\
image\_4  & 0.700 & 1.000 & 0.600 & 0.042 \\
image\_5  & 0.600 & 1.000 & 0.570 & 0.038 \\
image\_6  & 0.430 & 1.000 & 0.570 & 0.083 \\
image\_7  & 0.600 & 1.000 & 0.500 & 0.058 \\
image\_8  & 0.630 & 1.000 & 0.600 & 0.046 \\
image\_9  & 0.630 & 1.000 & 0.530 & 0.087 \\
image\_10 & 0.570 & 1.000 & 0.570 & 0.099 \\
image\_11 & 0.530 & 1.000 & 0.530 & 0.051 \\
image\_12 & 0.670 & 1.000 & 0.530 & 0.092 \\
image\_13 & 0.530 & 1.000 & 0.600 & 0.063 \\
image\_14 & 0.500 & 1.000 & 0.500 & 0.069 \\
image\_15 & 0.630 & 1.000 & 0.530 & 0.057 \\
image\_16 & 0.630 & 1.000 & 0.530 & 0.064 \\
image\_17 & 0.570 & 1.000 & 0.600 & 0.068 \\
image\_18 & 0.530 & 1.000 & 0.570 & 0.081 \\
image\_19 & 0.470 & 1.000 & 0.570 & 0.070 \\
image\_20 & 0.500 & 1.000 & 0.530 & 0.079 \\
image\_21 & 0.570 & 1.000 & 0.470 & 0.065 \\
image\_22 & 0.700 & 1.000 & 0.530 & 0.071 \\
image\_23 & 0.600 & 1.000 & 0.530 & 0.087 \\
image\_24 & 0.630 & 1.000 & 0.600 & 0.066 \\
image\_25 & 0.600 & 1.000 & 0.600 & 0.092 \\
image\_26 & 0.600 & 1.000 & 0.530 & 0.138 \\
image\_27 & 0.570 & 1.000 & 0.400 & 0.129 \\
image\_28 & 0.430 & 1.000 & 0.570 & 0.109 \\
image\_29 & 0.570 & 1.000 & 0.670 & 0.055 \\
image\_30 & 0.700 & 1.000 & 0.600 & 0.050 \\
image\_31 & 0.600 & 1.000 & 0.600 & 0.080 \\
image\_32 & 0.470 & 1.000 & 0.530 & 0.096 \\
image\_33 & 0.570 & 1.000 & 0.570 & 0.070 \\
image\_34 & 0.430 & 1.000 & 0.500 & 0.139 \\
image\_35 & 0.670 & 1.000 & 0.630 & 0.086 \\
image\_36 & 0.530 & 1.000 & 0.530 & 0.082 \\
image\_37 & 0.630 & 1.000 & 0.630 & 0.085 \\
image\_38 & 0.600 & 1.000 & 0.530 & 0.107 \\
image\_39 & 0.700 & 1.000 & 0.630 & 0.028 \\
image\_40 & 0.470 & 1.000 & 0.470 & 0.147 \\
image\_41 & 0.570 & 1.000 & 0.670 & 0.031 \\
image\_42 & 0.670 & 1.000 & 0.570 & 0.072 \\
image\_43 & 0.600 & 1.000 & 0.470 & 0.060 \\
image\_44 & 0.600 & 1.000 & 0.600 & 0.042 \\
image\_45 & 0.630 & 1.000 & 0.700 & 0.062 \\
image\_46 & 0.630 & 1.000 & 0.630 & 0.049 \\
image\_47 & 0.530 & 1.000 & 0.600 & 0.037 \\
image\_48 & 0.670 & 1.000 & 0.470 & 0.097 \\
image\_49 & 0.570 & 1.000 & 0.500 & 0.073 \\
image\_50 & 0.600 & 1.000 & 0.570 & 0.113 \\

\midrule
\textbf{Average (COCO, 1--25)}     & 0.581 & 1.000 & 0.549 & 0.070 \\
\textbf{Average (CelebA, 26--50)} & 0.584 & 1.000 & 0.567 & 0.082 \\

\end{longtable}
\endgroup



\begingroup
\small
\setlength{\tabcolsep}{4pt}
\renewcommand{\arraystretch}{0.95}

\begin{longtable}{lcccc}
\caption{Base StegaStamp attacked by \textbf{semantic attack}: per-image bit accuracy before watermarking ($\mathrm{BA}_{\text{orig}}$), after watermarking ($\mathrm{BA}_{\text{wm}}$), and after removal ($\mathrm{BA}_{\text{att}}$), with similarity score. Images 1--25: COCO, 26--50: CelebA.}
\label{tab:stega_base_semantic}\\
\toprule
Image & $\mathrm{BA}_{\text{orig}}$ & $\mathrm{BA}_{\text{wm}}$ & $\mathrm{BA}_{\text{att}}$ & Similarity Score \\
\midrule
\endfirsthead

\toprule
Image & $\mathrm{BA}_{\text{orig}}$ & $\mathrm{BA}_{\text{wm}}$ & $\mathrm{BA}_{\text{att}}$ & Similarity Score \\
\midrule
\endhead

\midrule
\multicolumn{5}{r}{\textit{Continued on next page}}\\
\endfoot

\bottomrule
\endlastfoot

image\_1  & 0.490 & 1.000 & 0.640 & 0.055 \\
image\_2  & 0.520 & 1.000 & 0.550 & 0.089 \\
image\_3  & 0.470 & 1.000 & 0.560 & 0.060 \\
image\_4  & 0.510 & 1.000 & 0.670 & 0.059 \\
image\_5  & 0.520 & 1.000 & 0.580 & 0.048 \\
image\_6  & 0.580 & 1.000 & 0.510 & 0.060 \\
image\_7  & 0.550 & 1.000 & 0.660 & 0.055 \\
image\_8  & 0.580 & 1.000 & 0.560 & 0.073 \\
image\_9  & 0.450 & 1.000 & 0.630 & 0.074 \\
image\_10 & 0.530 & 1.000 & 0.600 & 0.072 \\
image\_11 & 0.470 & 1.000 & 0.690 & 0.052 \\
image\_12 & 0.510 & 1.000 & 0.580 & 0.078 \\
image\_13 & 0.500 & 0.990 & 0.620 & 0.060 \\
image\_14 & 0.510 & 1.000 & 0.590 & 0.057 \\
image\_15 & 0.390 & 1.000 & 0.620 & 0.062 \\
image\_16 & 0.510 & 1.000 & 0.570 & 0.066 \\
image\_17 & 0.460 & 1.000 & 0.620 & 0.063 \\
image\_18 & 0.460 & 1.000 & 0.530 & 0.068 \\
image\_19 & 0.410 & 1.000 & 0.650 & 0.081 \\
image\_20 & 0.550 & 1.000 & 0.520 & 0.092 \\
image\_21 & 0.540 & 1.000 & 0.540 & 0.071 \\
image\_22 & 0.470 & 1.000 & 0.630 & 0.058 \\
image\_23 & 0.450 & 0.990 & 0.600 & 0.066 \\
image\_24 & 0.440 & 0.990 & 0.690 & 0.065 \\
image\_25 & 0.530 & 1.000 & 0.630 & 0.080 \\
image\_26 & 0.550 & 1.000 & 0.510 & 0.100 \\
image\_27 & 0.460 & 1.000 & 0.600 & 0.094 \\
image\_28 & 0.510 & 1.000 & 0.670 & 0.075 \\
image\_29 & 0.450 & 1.000 & 0.610 & 0.041 \\
image\_30 & 0.470 & 1.000 & 0.480 & 0.062 \\
image\_31 & 0.530 & 1.000 & 0.630 & 0.067 \\
image\_32 & 0.550 & 1.000 & 0.460 & 0.097 \\
image\_33 & 0.500 & 1.000 & 0.550 & 0.064 \\
image\_34 & 0.530 & 1.000 & 0.560 & 0.106 \\
image\_35 & 0.570 & 1.000 & 0.580 & 0.090 \\
image\_36 & 0.560 & 1.000 & 0.590 & 0.054 \\
image\_37 & 0.530 & 1.000 & 0.560 & 0.086 \\
image\_38 & 0.500 & 1.000 & 0.650 & 0.075 \\
image\_39 & 0.490 & 1.000 & 0.550 & 0.034 \\
image\_40 & 0.530 & 1.000 & 0.660 & 0.102 \\
image\_41 & 0.500 & 1.000 & 0.590 & 0.044 \\
image\_42 & 0.590 & 1.000 & 0.490 & 0.072 \\
image\_43 & 0.540 & 1.000 & 0.600 & 0.058 \\
image\_44 & 0.540 & 1.000 & 0.520 & 0.057 \\
image\_45 & 0.560 & 1.000 & 0.520 & 0.051 \\
image\_46 & 0.500 & 1.000 & 0.540 & 0.061 \\
image\_47 & 0.560 & 1.000 & 0.600 & 0.048 \\
image\_48 & 0.540 & 1.000 & 0.460 & 0.109 \\
image\_49 & 0.480 & 1.000 & 0.550 & 0.071 \\
image\_50 & 0.470 & 1.000 & 0.550 & 0.085 \\

\midrule
\textbf{Average (COCO, 1--25)}     & 0.496 & 0.999 & 0.602 & 0.067 \\
\textbf{Average (CelebA, 26--50)} & 0.520 & 1.000 & 0.563 & 0.072 \\

\end{longtable}
\endgroup

\subsection{Phase 2: Dual watermarking study}
\begingroup
\small
\setlength{\tabcolsep}{4pt}
\renewcommand{\arraystretch}{0.95}

\begin{longtable}{lccc}
\caption{Phase 2 (HiDDeNStega) --- Step 1: HiDDeN embedding on the benchmark dataset. Per-image bit accuracy for each decoder: $\mathrm{BA}_{\text{HiDDeN}}$ and $\mathrm{BA}_{\text{Stega}}$, with similarity score. Images 1--25: COCO, 26--50: CelebA.}
\label{tab:phase1_hiddenstega_step1_hidden_embed}\\
\toprule
Image & $\mathrm{BA}_{\text{HiDDeN}}$ & $\mathrm{BA}_{\text{Stega}}$ & Similarity Score \\
\midrule
\endfirsthead

\toprule
Image & $\mathrm{BA}_{\text{HiDDeN}}$ & $\mathrm{BA}_{\text{Stega}}$ & Similarity Score \\
\midrule
\endhead

\midrule
\multicolumn{4}{r}{\textit{Continued on next page}}\\
\endfoot

\bottomrule
\endlastfoot

image\_1.png  & 1.000 & 0.530 & 0.026 \\
image\_2.png  & 1.000 & 0.560 & 0.073 \\
image\_3.png  & 1.000 & 0.430 & 0.039 \\
image\_4.png  & 1.000 & 0.500 & 0.026 \\
image\_5.png  & 1.000 & 0.530 & 0.024 \\
image\_6.png  & 1.000 & 0.520 & 0.059 \\
image\_7.png  & 1.000 & 0.570 & 0.024 \\
image\_8.png  & 0.970 & 0.610 & 0.041 \\
image\_9.png  & 1.000 & 0.500 & 0.046 \\
image\_10.png & 1.000 & 0.570 & 0.043 \\
image\_11.png & 1.000 & 0.420 & 0.027 \\
image\_12.png & 1.000 & 0.500 & 0.051 \\
image\_13.png & 1.000 & 0.570 & 0.028 \\
image\_14.png & 1.000 & 0.500 & 0.029 \\
image\_15.png & 1.000 & 0.470 & 0.033 \\
image\_16.png & 1.000 & 0.500 & 0.031 \\
image\_17.png & 1.000 & 0.430 & 0.034 \\
image\_18.png & 1.000 & 0.470 & 0.034 \\
image\_19.png & 1.000 & 0.450 & 0.044 \\
image\_20.png & 0.970 & 0.520 & 0.049 \\
image\_21.png & 1.000 & 0.570 & 0.036 \\
image\_22.png & 1.000 & 0.480 & 0.035 \\
image\_23.png & 1.000 & 0.420 & 0.038 \\
image\_24.png & 1.000 & 0.470 & 0.028 \\
image\_25.png & 1.000 & 0.480 & 0.049 \\
image\_26.png & 1.000 & 0.550 & 0.073 \\
image\_27.png & 1.000 & 0.540 & 0.089 \\
image\_28.png & 1.000 & 0.490 & 0.050 \\
image\_29.png & 1.000 & 0.490 & 0.068 \\
image\_30.png & 1.000 & 0.460 & 0.037 \\
image\_31.png & 1.000 & 0.500 & 0.041 \\
image\_32.png & 1.000 & 0.470 & 0.070 \\
image\_33.png & 1.000 & 0.570 & 0.037 \\
image\_34.png & 1.000 & 0.490 & 0.080 \\
image\_35.png & 1.000 & 0.540 & 0.062 \\
image\_36.png & 1.000 & 0.520 & 0.055 \\
image\_37.png & 1.000 & 0.580 & 0.041 \\
image\_38.png & 1.000 & 0.560 & 0.062 \\
image\_39.png & 1.000 & 0.500 & 0.034 \\
image\_40.png & 0.930 & 0.550 & 0.084 \\
image\_41.png & 0.970 & 0.550 & 0.028 \\
image\_42.png & 1.000 & 0.570 & 0.038 \\
image\_43.png & 1.000 & 0.530 & 0.040 \\
image\_44.png & 1.000 & 0.540 & 0.020 \\
image\_45.png & 1.000 & 0.600 & 0.040 \\
image\_46.png & 1.000 & 0.490 & 0.029 \\
image\_47.png & 0.970 & 0.500 & 0.028 \\
image\_48.png & 1.000 & 0.500 & 0.067 \\
image\_49.png & 1.000 & 0.520 & 0.077 \\
image\_50.png & 0.970 & 0.460 & 0.055 \\

\midrule
\textbf{Average (COCO, 1--25)}     & 0.998 & 0.503 & 0.038 \\
\textbf{Average (CelebA, 26--50)} & 0.994 & 0.523 & 0.052 \\

\end{longtable}
\endgroup


\begingroup
\small
\setlength{\tabcolsep}{4pt}
\renewcommand{\arraystretch}{0.95}

\begin{longtable}{lccc}
\caption{Phase 2 (HiDDeNStega) --- Step 2: StegaStamp embedding on the HiDDeN-embedded dataset to create \textit{HiDDeNStega}. Per-image bit accuracy for each decoder: $\mathrm{BA}_{\text{HiDDeN}}$ and $\mathrm{BA}_{\text{Stega}}$, with similarity score. Images 1--25: COCO, 26--50: CelebA.}
\label{tab:phase1_hiddenstega_step2_stega_embed}\\
\toprule
Image & $\mathrm{BA}_{\text{HiDDeN}}$ & $\mathrm{BA}_{\text{Stega}}$ & Similarity Score \\
\midrule
\endfirsthead

\toprule
Image & $\mathrm{BA}_{\text{HiDDeN}}$ & $\mathrm{BA}_{\text{Stega}}$ & Similarity Score \\
\midrule
\endhead

\midrule
\multicolumn{4}{r}{\textit{Continued on next page}}\\
\endfoot

\bottomrule
\endlastfoot

image\_1.png  & 1.000 & 0.980 & 0.141 \\
image\_2.png  & 0.930 & 0.980 & 0.199 \\
image\_3.png  & 0.970 & 0.990 & 0.131 \\
image\_4.png  & 1.000 & 0.980 & 0.128 \\
image\_5.png  & 1.000 & 0.980 & 0.120 \\
image\_6.png  & 0.930 & 0.980 & 0.157 \\
image\_7.png  & 1.000 & 0.980 & 0.105 \\
image\_8.png  & 0.930 & 0.980 & 0.077 \\
image\_9.png  & 1.000 & 0.980 & 0.133 \\
image\_10.png & 1.000 & 0.980 & 0.227 \\
image\_11.png & 1.000 & 0.980 & 0.143 \\
image\_12.png & 1.000 & 0.990 & 0.135 \\
image\_13.png & 0.970 & 0.980 & 0.122 \\
image\_14.png & 1.000 & 0.980 & 0.124 \\
image\_15.png & 0.870 & 0.980 & 0.156 \\
image\_16.png & 1.000 & 0.990 & 0.141 \\
image\_17.png & 1.000 & 0.980 & 0.122 \\
image\_18.png & 1.000 & 0.980 & 0.150 \\
image\_19.png & 1.000 & 0.980 & 0.108 \\
image\_20.png & 0.970 & 0.980 & 0.153 \\
image\_21.png & 0.970 & 0.980 & 0.117 \\
image\_22.png & 1.000 & 0.990 & 0.142 \\
image\_23.png & 0.900 & 0.980 & 0.226 \\
image\_24.png & 1.000 & 0.980 & 0.093 \\
image\_25.png & 0.970 & 0.980 & 0.200 \\
image\_26.png & 1.000 & 0.980 & 0.128 \\
image\_27.png & 1.000 & 0.980 & 0.092 \\
image\_28.png & 1.000 & 0.980 & 0.113 \\
image\_29.png & 1.000 & 0.980 & 0.109 \\
image\_30.png & 0.930 & 0.980 & 0.088 \\
image\_31.png & 1.000 & 0.980 & 0.069 \\
image\_32.png & 1.000 & 0.980 & 0.087 \\
image\_33.png & 0.970 & 0.980 & 0.116 \\
image\_34.png & 0.970 & 0.980 & 0.207 \\
image\_35.png & 1.000 & 0.980 & 0.114 \\
image\_36.png & 1.000 & 0.990 & 0.116 \\
image\_37.png & 1.000 & 0.980 & 0.117 \\
image\_38.png & 1.000 & 0.980 & 0.112 \\
image\_39.png & 1.000 & 0.980 & 0.055 \\
image\_40.png & 0.900 & 0.980 & 0.127 \\
image\_41.png & 0.970 & 0.980 & 0.048 \\
image\_42.png & 1.000 & 0.980 & 0.092 \\
image\_43.png & 1.000 & 0.980 & 0.110 \\
image\_44.png & 1.000 & 0.980 & 0.062 \\
image\_45.png & 1.000 & 0.980 & 0.129 \\
image\_46.png & 1.000 & 0.980 & 0.064 \\
image\_47.png & 0.970 & 0.990 & 0.075 \\
image\_48.png & 0.970 & 0.990 & 0.180 \\
image\_49.png & 1.000 & 0.980 & 0.069 \\
image\_50.png & 0.970 & 0.980 & 0.098 \\

\midrule
\textbf{Average (COCO, 1--25)}     & 0.976 & 0.982 & 0.142 \\
\textbf{Average (CelebA, 26--50)} & 0.986 & 0.981 & 0.103 \\

\end{longtable}
\endgroup

\begingroup
\small
\setlength{\tabcolsep}{4pt}
\renewcommand{\arraystretch}{0.95}

\begin{longtable}{lccc}
\caption{Phase 2 (StegaHiDDeN) --- Step 1: StegaStamp embedding on the benchmark dataset. Per-image bit accuracy for each decoder: $\mathrm{BA}_{\text{HiDDeN}}$ (hidden) and $\mathrm{BA}_{\text{Stega}}$ (stega), with similarity score. Images 1--25: COCO, 26--50: CelebA.}
\label{tab:phase1_stegahidden_step1_stega_embed}\\
\toprule
Image & $\mathrm{BA}_{\text{HiDDeN}}$ & $\mathrm{BA}_{\text{Stega}}$ & Similarity Score \\
\midrule
\endfirsthead

\toprule
Image & $\mathrm{BA}_{\text{HiDDeN}}$ & $\mathrm{BA}_{\text{Stega}}$ & Similarity Score \\
\midrule
\endhead

\midrule
\multicolumn{4}{r}{\textit{Continued on next page}}\\
\endfoot

\bottomrule
\endlastfoot

image\_1.png  & 0.570 & 1.000 & 0.145 \\
image\_2.png  & 0.430 & 1.000 & 0.220 \\
image\_3.png  & 0.330 & 1.000 & 0.219 \\
image\_4.png  & 0.530 & 1.000 & 0.147 \\
image\_5.png  & 0.400 & 1.000 & 0.139 \\
image\_6.png  & 0.370 & 1.000 & 0.192 \\
image\_7.png  & 0.470 & 1.000 & 0.126 \\
image\_8.png  & 0.470 & 1.000 & 0.155 \\
image\_9.png  & 0.430 & 1.000 & 0.218 \\
image\_10.png & 0.370 & 1.000 & 0.221 \\
image\_11.png & 0.400 & 1.000 & 0.148 \\
image\_12.png & 0.400 & 1.000 & 0.196 \\
image\_13.png & 0.400 & 0.990 & 0.135 \\
image\_14.png & 0.500 & 1.000 & 0.158 \\
image\_15.png & 0.430 & 1.000 & 0.191 \\
image\_16.png & 0.400 & 1.000 & 0.192 \\
image\_17.png & 0.400 & 1.000 & 0.148 \\
image\_18.png & 0.400 & 1.000 & 0.174 \\
image\_19.png & 0.430 & 1.000 & 0.170 \\
image\_20.png & 0.370 & 1.000 & 0.255 \\
image\_21.png & 0.430 & 1.000 & 0.178 \\
image\_22.png & 0.500 & 1.000 & 0.185 \\
image\_23.png & 0.430 & 0.990 & 0.192 \\
image\_24.png & 0.530 & 0.990 & 0.147 \\
image\_25.png & 0.400 & 1.000 & 0.222 \\
image\_26.png & 0.470 & 1.000 & 0.172 \\
image\_27.png & 0.400 & 1.000 & 0.186 \\
image\_28.png & 0.670 & 1.000 & 0.147 \\
image\_29.png & 0.430 & 1.000 & 0.141 \\
image\_30.png & 0.570 & 1.000 & 0.107 \\
image\_31.png & 0.430 & 1.000 & 0.125 \\
image\_32.png & 0.400 & 1.000 & 0.184 \\
image\_33.png & 0.430 & 1.000 & 0.122 \\
image\_34.png & 0.400 & 1.000 & 0.215 \\
image\_35.png & 0.470 & 1.000 & 0.125 \\
image\_36.png & 0.470 & 1.000 & 0.166 \\
image\_37.png & 0.500 & 1.000 & 0.132 \\
image\_38.png & 0.470 & 1.000 & 0.231 \\
image\_39.png & 0.500 & 1.000 & 0.104 \\
image\_40.png & 0.400 & 1.000 & 0.247 \\
image\_41.png & 0.530 & 1.000 & 0.091 \\
image\_42.png & 0.370 & 1.000 & 0.113 \\
image\_43.png & 0.500 & 1.000 & 0.134 \\
image\_44.png & 0.500 & 1.000 & 0.093 \\
image\_45.png & 0.470 & 1.000 & 0.124 \\
image\_46.png & 0.400 & 1.000 & 0.096 \\
image\_47.png & 0.500 & 1.000 & 0.086 \\
image\_48.png & 0.470 & 1.000 & 0.187 \\
image\_49.png & 0.400 & 1.000 & 0.139 \\
image\_50.png & 0.400 & 1.000 & 0.173 \\

\midrule
\textbf{Average (COCO, 1--25)}     & 0.437 & 0.998 & 0.179 \\
\textbf{Average (CelebA, 26--50)} & 0.459 & 1.000 & 0.145 \\

\end{longtable}
\endgroup



\begingroup
\small
\setlength{\tabcolsep}{4pt}
\renewcommand{\arraystretch}{0.95}

\begin{longtable}{lccc}
\caption{Phase 2 (StegaHiDDeN) --- Step 2: HiDDeN embedding on the StegaStamp-embedded dataset to create \textit{StegaHiDDeN}. Per-image bit accuracy for each decoder: $\mathrm{BA}_{\text{HiDDeN}}$ and $\mathrm{BA}_{\text{Stega}}$, with similarity score. Images 1--25: COCO, 26--50: CelebA.}
\label{tab:phase1_stegahidden_step2_hidden_embed}\\
\toprule
Image & $\mathrm{BA}_{\text{HiDDeN}}$ & $\mathrm{BA}_{\text{Stega}}$ & Similarity Score \\
\midrule
\endfirsthead

\toprule
Image & $\mathrm{BA}_{\text{HiDDeN}}$ & $\mathrm{BA}_{\text{Stega}}$ & Similarity Score \\
\midrule
\endhead

\midrule
\multicolumn{4}{r}{\textit{Continued on next page}}\\
\endfoot

\bottomrule
\endlastfoot

image\_1.png  & 1.000 & 0.980 & 0.026 \\
image\_2.png  & 1.000 & 0.990 & 0.057 \\
image\_3.png  & 1.000 & 1.000 & 0.035 \\
image\_4.png  & 1.000 & 0.980 & 0.032 \\
image\_5.png  & 1.000 & 0.990 & 0.027 \\
image\_6.png  & 1.000 & 1.000 & 0.042 \\
image\_7.png  & 1.000 & 1.000 & 0.023 \\
image\_8.png  & 1.000 & 1.000 & 0.037 \\
image\_9.png  & 1.000 & 1.000 & 0.042 \\
image\_10.png & 1.000 & 1.000 & 0.041 \\
image\_11.png & 1.000 & 0.990 & 0.031 \\
image\_12.png & 1.000 & 1.000 & 0.037 \\
image\_13.png & 1.000 & 0.990 & 0.034 \\
image\_14.png & 1.000 & 1.000 & 0.032 \\
image\_15.png & 1.000 & 0.990 & 0.031 \\
image\_16.png & 1.000 & 1.000 & 0.032 \\
image\_17.png & 1.000 & 0.970 & 0.028 \\
image\_18.png & 1.000 & 1.000 & 0.036 \\
image\_19.png & 1.000 & 1.000 & 0.042 \\
image\_20.png & 1.000 & 1.000 & 0.043 \\
image\_21.png & 1.000 & 1.000 & 0.035 \\
image\_22.png & 1.000 & 0.980 & 0.042 \\
image\_23.png & 1.000 & 0.980 & 0.040 \\
image\_24.png & 1.000 & 1.000 & 0.029 \\
image\_25.png & 1.000 & 1.000 & 0.041 \\
image\_26.png & 1.000 & 1.000 & 0.071 \\
image\_27.png & 1.000 & 0.990 & 0.065 \\
image\_28.png & 1.000 & 0.990 & 0.042 \\
image\_29.png & 1.000 & 0.980 & 0.066 \\
image\_30.png & 1.000 & 0.990 & 0.032 \\
image\_31.png & 1.000 & 1.000 & 0.041 \\
image\_32.png & 1.000 & 1.000 & 0.057 \\
image\_33.png & 1.000 & 0.980 & 0.043 \\
image\_34.png & 1.000 & 0.980 & 0.062 \\
image\_35.png & 1.000 & 0.980 & 0.056 \\
image\_36.png & 1.000 & 1.000 & 0.058 \\
image\_37.png & 1.000 & 0.980 & 0.036 \\
image\_38.png & 1.000 & 1.000 & 0.051 \\
image\_39.png & 0.970 & 1.000 & 0.032 \\
image\_40.png & 1.000 & 1.000 & 0.092 \\
image\_41.png & 0.970 & 1.000 & 0.026 \\
image\_42.png & 1.000 & 1.000 & 0.035 \\
image\_43.png & 1.000 & 0.990 & 0.037 \\
image\_44.png & 1.000 & 0.990 & 0.025 \\
image\_45.png & 1.000 & 1.000 & 0.038 \\
image\_46.png & 1.000 & 0.980 & 0.028 \\
image\_47.png & 0.970 & 0.980 & 0.026 \\
image\_48.png & 1.000 & 1.000 & 0.076 \\
image\_49.png & 0.970 & 1.000 & 0.059 \\
image\_50.png & 1.000 & 1.000 & 0.051 \\

\midrule
\textbf{Average (COCO, 1--25)}     & 1.000 & 0.994 & 0.035 \\
\textbf{Average (CelebA, 26--50)} & 0.993 & 0.992 & 0.052 \\

\end{longtable}


\endgroup

\subsection{Phase 3: Dual attack sequence study}
\begingroup
\small
\setlength{\tabcolsep}{4pt}
\renewcommand{\arraystretch}{0.95}

\begin{longtable}{lccc}
\caption{Non-semantic attack on \textit{HiDDeNStega} dataset. Per-image bit accuracy for each decoder: $\mathrm{BA}_{\text{HiDDeN}}$ and $\mathrm{BA}_{\text{Stega}}$, with LPIPS (Similarity Score). Images 1--25: COCO, 26--50: CelebA.}
\label{tab:P3_HS_NS}\\
\toprule
Image & $\mathrm{BA}_{\text{HiDDeN}}$ & $\mathrm{BA}_{\text{Stega}}$ & LPIPS \\
\midrule
\endfirsthead

\toprule
Image & $\mathrm{BA}_{\text{HiDDeN}}$ & $\mathrm{BA}_{\text{Stega}}$ & LPIPS \\
\midrule
\endhead

\midrule
\multicolumn{4}{r}{\textit{Continued on next page}}\\
\endfoot

\bottomrule
\endlastfoot

image\_1.png  & 0.600 & 0.940 & 0.007 \\
image\_2.png  & 0.600 & 0.960 & 0.012 \\
image\_3.png  & 0.530 & 0.940 & 0.008 \\
image\_4.png  & 0.770 & 0.930 & 0.008 \\
image\_5.png  & 0.530 & 0.980 & 0.006 \\
image\_6.png  & 0.600 & 0.970 & 0.008 \\
image\_7.png  & 0.630 & 0.970 & 0.007 \\
image\_8.png  & 0.630 & 0.960 & 0.009 \\
image\_9.png  & 0.600 & 0.920 & 0.010 \\
image\_10.png & 0.670 & 0.960 & 0.010 \\
image\_11.png & 0.570 & 0.960 & 0.009 \\
image\_12.png & 0.600 & 0.960 & 0.010 \\
image\_13.png & 0.570 & 0.970 & 0.008 \\
image\_14.png & 0.530 & 0.980 & 0.008 \\
image\_15.png & 0.470 & 0.980 & 0.008 \\
image\_16.png & 0.600 & 0.940 & 0.008 \\
image\_17.png & 0.500 & 0.960 & 0.007 \\
image\_18.png & 0.600 & 0.950 & 0.009 \\
image\_19.png & 0.600 & 0.950 & 0.011 \\
image\_20.png & 0.570 & 0.950 & 0.009 \\
image\_21.png & 0.630 & 0.970 & 0.008 \\
image\_22.png & 0.570 & 0.970 & 0.008 \\
image\_23.png & 0.500 & 0.850 & 0.008 \\
image\_24.png & 0.570 & 0.950 & 0.008 \\
image\_25.png & 0.570 & 0.980 & 0.008 \\
image\_26.png & 0.530 & 0.970 & 0.014 \\
image\_27.png & 0.630 & 0.890 & 0.010 \\
image\_28.png & 0.530 & 0.970 & 0.009 \\
image\_29.png & 0.770 & 0.990 & 0.008 \\
image\_30.png & 0.500 & 0.970 & 0.008 \\
image\_31.png & 0.570 & 0.950 & 0.012 \\
image\_32.png & 0.700 & 0.910 & 0.011 \\
image\_33.png & 0.570 & 0.980 & 0.011 \\
image\_34.png & 0.600 & 0.970 & 0.009 \\
image\_35.png & 0.700 & 0.990 & 0.011 \\
image\_36.png & 0.730 & 0.900 & 0.008 \\
image\_37.png & 0.500 & 0.970 & 0.013 \\
image\_38.png & 0.530 & 0.950 & 0.011 \\
image\_39.png & 0.600 & 0.960 & 0.005 \\
image\_40.png & 0.530 & 0.970 & 0.011 \\
image\_41.png & 0.670 & 0.950 & 0.007 \\
image\_42.png & 0.630 & 0.970 & 0.011 \\
image\_43.png & 0.570 & 0.980 & 0.010 \\
image\_44.png & 0.670 & 0.970 & 0.011 \\
image\_45.png & 0.730 & 0.970 & 0.007 \\
image\_46.png & 0.600 & 0.960 & 0.011 \\
image\_47.png & 0.730 & 0.960 & 0.008 \\
image\_48.png & 0.570 & 1.000 & 0.016 \\
image\_49.png & 0.630 & 0.970 & 0.007 \\
image\_50.png & 0.570 & 0.930 & 0.012 \\

\midrule
\textbf{Average (COCO, 1--25)}     & 0.584 & 0.954 & 0.009 \\
\textbf{Average (CelebA, 26--50)} & 0.614 & 0.960 & 0.010 \\
\textbf{Average (Overall, 1--50)} & 0.599 & 0.957 & 0.009 \\

\end{longtable}
\endgroup


\begingroup
\small
\setlength{\tabcolsep}{4pt}
\renewcommand{\arraystretch}{0.95}

\begin{longtable}{lccc}
\caption{Semantic attack on the \textit{HiDDeNStega} dataset \textbf{after} a non-semantic attack (i.e., Non-semantic $\rightarrow$ semantic). Per-image bit accuracy for each decoder: $\mathrm{BA}_{\text{HiDDeN}}$ and $\mathrm{BA}_{\text{Stega}}$, with LPIPS (Similarity Score). Images 1--25: COCO, 26--50: CelebA.}
\label{tab:p3_HS_NS_S}\\
\toprule
Image & $\mathrm{BA}_{\text{HiDDeN}}$ & $\mathrm{BA}_{\text{Stega}}$ & LPIPS \\
\midrule
\endfirsthead

\toprule
Image & $\mathrm{BA}_{\text{HiDDeN}}$ & $\mathrm{BA}_{\text{Stega}}$ & LPIPS \\
\midrule
\endhead

\midrule
\multicolumn{4}{r}{\textit{Continued on next page}}\\
\endfoot

\bottomrule
\endlastfoot

image\_1.png  & 0.630 & 0.640 & 0.071 \\
image\_2.png  & 0.600 & 0.650 & 0.111 \\
image\_3.png  & 0.430 & 0.690 & 0.067 \\
image\_4.png  & 0.700 & 0.820 & 0.068 \\
image\_5.png  & 0.530 & 0.750 & 0.055 \\
image\_6.png  & 0.530 & 0.740 & 0.086 \\
image\_7.png  & 0.600 & 0.770 & 0.068 \\
image\_8.png  & 0.630 & 0.790 & 0.065 \\
image\_9.png  & 0.570 & 0.670 & 0.096 \\
image\_10.png & 0.600 & 0.800 & 0.098 \\
image\_11.png & 0.530 & 0.750 & 0.071 \\
image\_12.png & 0.570 & 0.710 & 0.084 \\
image\_13.png & 0.500 & 0.640 & 0.066 \\
image\_14.png & 0.530 & 0.810 & 0.069 \\
image\_15.png & 0.470 & 0.690 & 0.086 \\
image\_16.png & 0.570 & 0.770 & 0.078 \\
image\_17.png & 0.430 & 0.680 & 0.087 \\
image\_18.png & 0.500 & 0.650 & 0.088 \\
image\_19.png & 0.530 & 0.630 & 0.100 \\
image\_20.png & 0.530 & 0.780 & 0.090 \\
image\_21.png & 0.600 & 0.760 & 0.083 \\
image\_22.png & 0.570 & 0.790 & 0.087 \\
image\_23.png & 0.530 & 0.710 & 0.083 \\
image\_24.png & 0.600 & 0.620 & 0.078 \\
image\_25.png & 0.570 & 0.690 & 0.101 \\
image\_26.png & 0.530 & 0.480 & 0.112 \\
image\_27.png & 0.600 & 0.530 & 0.105 \\
image\_28.png & 0.530 & 0.720 & 0.065 \\
image\_29.png & 0.670 & 0.680 & 0.083 \\
image\_30.png & 0.530 & 0.700 & 0.064 \\
image\_31.png & 0.600 & 0.580 & 0.097 \\
image\_32.png & 0.630 & 0.600 & 0.089 \\
image\_33.png & 0.570 & 0.640 & 0.091 \\
image\_34.png & 0.630 & 0.890 & 0.116 \\
image\_35.png & 0.630 & 0.560 & 0.103 \\
image\_36.png & 0.700 & 0.660 & 0.076 \\
image\_37.png & 0.470 & 0.710 & 0.092 \\
image\_38.png & 0.530 & 0.640 & 0.102 \\
image\_39.png & 0.600 & 0.930 & 0.033 \\
image\_40.png & 0.470 & 0.660 & 0.122 \\
image\_41.png & 0.670 & 0.650 & 0.048 \\
image\_42.png & 0.600 & 0.640 & 0.084 \\
image\_43.png & 0.570 & 0.580 & 0.085 \\
image\_44.png & 0.600 & 0.740 & 0.065 \\
image\_45.png & 0.730 & 0.670 & 0.062 \\
image\_46.png & 0.600 & 0.600 & 0.073 \\
image\_47.png & 0.670 & 0.790 & 0.061 \\
image\_48.png & 0.530 & 0.670 & 0.139 \\
image\_49.png & 0.630 & 0.610 & 0.080 \\
image\_50.png & 0.530 & 0.500 & 0.081 \\

\midrule
\textbf{Average (COCO, 1--25)}     & 0.554 & 0.720 & 0.081 \\
\textbf{Average (CelebA, 26--50)} & 0.593 & 0.657 & 0.085 \\
\textbf{Average (Overall, 1--50)} & 0.573 & 0.689 & 0.083 \\

\end{longtable}
\endgroup


\begingroup
\small
\setlength{\tabcolsep}{4pt}
\renewcommand{\arraystretch}{0.95}

\begin{longtable}{lccc}
\caption{Semantic attack on \textit{HiDDeNStega} dataset. Per-image bit accuracy for each decoder: $\mathrm{BA}_{\text{HiDDeN}}$ and $\mathrm{BA}_{\text{Stega}}$, with LPIPS (Similarity Score). Images 1--25: COCO, 26--50: CelebA.}
\label{tab:P3_HS_S}\\
\toprule
Image & $\mathrm{BA}_{\text{HiDDeN}}$ & $\mathrm{BA}_{\text{Stega}}$ & LPIPS \\
\midrule
\endfirsthead

\toprule
Image & $\mathrm{BA}_{\text{HiDDeN}}$ & $\mathrm{BA}_{\text{Stega}}$ & LPIPS \\
\midrule
\endhead

\midrule
\multicolumn{4}{r}{\textit{Continued on next page}}\\
\endfoot

\bottomrule
\endlastfoot

image\_1.png  & 0.900 & 0.610 & 0.075 \\
image\_2.png  & 0.670 & 0.630 & 0.116 \\
image\_3.png  & 0.830 & 0.640 & 0.076 \\
image\_4.png  & 1.000 & 0.730 & 0.075 \\
image\_5.png  & 0.900 & 0.790 & 0.061 \\
image\_6.png  & 0.900 & 0.700 & 0.090 \\
image\_7.png  & 0.930 & 0.760 & 0.072 \\
image\_8.png  & 0.870 & 0.730 & 0.068 \\
image\_9.png  & 0.870 & 0.580 & 0.106 \\
image\_10.png & 0.870 & 0.750 & 0.101 \\
image\_11.png & 0.900 & 0.680 & 0.079 \\
image\_12.png & 0.830 & 0.610 & 0.094 \\
image\_13.png & 0.800 & 0.640 & 0.076 \\
image\_14.png & 0.870 & 0.700 & 0.079 \\
image\_15.png & 0.700 & 0.730 & 0.087 \\
image\_16.png & 0.900 & 0.690 & 0.084 \\
image\_17.png & 0.800 & 0.660 & 0.092 \\
image\_18.png & 0.870 & 0.620 & 0.094 \\
image\_19.png & 0.900 & 0.630 & 0.102 \\
image\_20.png & 0.830 & 0.700 & 0.097 \\
image\_21.png & 0.870 & 0.700 & 0.087 \\
image\_22.png & 0.900 & 0.680 & 0.092 \\
image\_23.png & 0.770 & 0.640 & 0.090 \\
image\_24.png & 0.930 & 0.590 & 0.086 \\
image\_25.png & 0.830 & 0.580 & 0.102 \\
image\_26.png & 0.930 & 0.580 & 0.094 \\
image\_27.png & 0.930 & 0.580 & 0.079 \\
image\_28.png & 0.870 & 0.560 & 0.064 \\
image\_29.png & 0.970 & 0.620 & 0.087 \\
image\_30.png & 0.930 & 0.580 & 0.065 \\
image\_31.png & 0.970 & 0.550 & 0.076 \\
image\_32.png & 0.900 & 0.580 & 0.066 \\
image\_33.png & 0.870 & 0.610 & 0.097 \\
image\_34.png & 0.830 & 0.880 & 0.120 \\
image\_35.png & 0.930 & 0.580 & 0.082 \\
image\_36.png & 0.900 & 0.630 & 0.083 \\
image\_37.png & 0.970 & 0.580 & 0.083 \\
image\_38.png & 0.900 & 0.650 & 0.112 \\
image\_39.png & 0.930 & 0.810 & 0.041 \\
image\_40.png & 0.730 & 0.570 & 0.109 \\
image\_41.png & 0.970 & 0.650 & 0.058 \\
image\_42.png & 0.930 & 0.570 & 0.072 \\
image\_43.png & 1.000 & 0.580 & 0.064 \\
image\_44.png & 0.930 & 0.610 & 0.073 \\
image\_45.png & 0.930 & 0.570 & 0.055 \\
image\_46.png & 0.970 & 0.580 & 0.066 \\
image\_47.png & 0.900 & 0.680 & 0.071 \\
image\_48.png & 0.700 & 0.580 & 0.123 \\
image\_49.png & 0.870 & 0.580 & 0.073 \\
image\_50.png & 0.970 & 0.570 & 0.078 \\

\midrule
\textbf{Average (COCO, 1--25)}     & 0.858 & 0.671 & 0.087 \\
\textbf{Average (CelebA, 26--50)} & 0.909 & 0.613 & 0.080 \\
\textbf{Average (Overall, 1--50)} & 0.883 & 0.642 & 0.083 \\

\end{longtable}
\endgroup


\begingroup
\small
\setlength{\tabcolsep}{4pt}
\renewcommand{\arraystretch}{0.95}

\begin{longtable}{lccc}
\caption{Non-semantic attack on the \textit{HiDDeNStega} dataset \textbf{after} a semantic attack (i.e., Semantic $\rightarrow$ Non-semantic). Per-image bit accuracy for each decoder: $\mathrm{BA}_{\text{HiDDeN}}$ and $\mathrm{BA}_{\text{Stega}}$, with LPIPS (Similarity Score). Images 1--25: COCO, 26--50: CelebA.}
\label{tab:P3_HS_S_NS}\\
\toprule
Image & $\mathrm{BA}_{\text{HiDDeN}}$ & $\mathrm{BA}_{\text{Stega}}$ & LPIPS \\
\midrule
\endfirsthead

\toprule
Image & $\mathrm{BA}_{\text{HiDDeN}}$ & $\mathrm{BA}_{\text{Stega}}$ & LPIPS \\
\midrule
\endhead

\midrule
\multicolumn{4}{r}{\textit{Continued on next page}}\\
\endfoot

\bottomrule
\endlastfoot

image\_1.png  & 0.630 & 0.660 & 0.007 \\
image\_2.png  & 0.570 & 0.650 & 0.008 \\
image\_3.png  & 0.570 & 0.680 & 0.006 \\
image\_4.png  & 0.730 & 0.740 & 0.008 \\
image\_5.png  & 0.600 & 0.760 & 0.006 \\
image\_6.png  & 0.570 & 0.730 & 0.006 \\
image\_7.png  & 0.600 & 0.730 & 0.007 \\
image\_8.png  & 0.670 & 0.690 & 0.009 \\
image\_9.png  & 0.570 & 0.590 & 0.007 \\
image\_10.png & 0.570 & 0.780 & 0.006 \\
image\_11.png & 0.570 & 0.730 & 0.007 \\
image\_12.png & 0.570 & 0.620 & 0.007 \\
image\_13.png & 0.570 & 0.630 & 0.006 \\
image\_14.png & 0.570 & 0.770 & 0.006 \\
image\_15.png & 0.570 & 0.700 & 0.005 \\
image\_16.png & 0.600 & 0.700 & 0.008 \\
image\_17.png & 0.570 & 0.620 & 0.003 \\
image\_18.png & 0.570 & 0.600 & 0.006 \\
image\_19.png & 0.630 & 0.600 & 0.010 \\
image\_20.png & 0.570 & 0.750 & 0.007 \\
image\_21.png & 0.530 & 0.720 & 0.007 \\
image\_22.png & 0.630 & 0.740 & 0.008 \\
image\_23.png & 0.600 & 0.720 & 0.008 \\
image\_24.png & 0.570 & 0.540 & 0.007 \\
image\_25.png & 0.570 & 0.630 & 0.006 \\
image\_26.png & 0.570 & 0.600 & 0.012 \\
image\_27.png & 0.600 & 0.590 & 0.010 \\
image\_28.png & 0.570 & 0.610 & 0.006 \\
image\_29.png & 0.670 & 0.630 & 0.007 \\
image\_30.png & 0.570 & 0.580 & 0.008 \\
image\_31.png & 0.630 & 0.610 & 0.013 \\
image\_32.png & 0.700 & 0.670 & 0.011 \\
image\_33.png & 0.570 & 0.590 & 0.007 \\
image\_34.png & 0.570 & 0.870 & 0.009 \\
image\_35.png & 0.630 & 0.610 & 0.012 \\
image\_36.png & 0.670 & 0.720 & 0.007 \\
image\_37.png & 0.570 & 0.610 & 0.008 \\
image\_38.png & 0.570 & 0.630 & 0.008 \\
image\_39.png & 0.670 & 0.850 & 0.005 \\
image\_40.png & 0.570 & 0.640 & 0.005 \\
image\_41.png & 0.700 & 0.670 & 0.007 \\
image\_42.png & 0.630 & 0.580 & 0.011 \\
image\_43.png & 0.630 & 0.610 & 0.011 \\
image\_44.png & 0.700 & 0.600 & 0.011 \\
image\_45.png & 0.700 & 0.610 & 0.007 \\
image\_46.png & 0.630 & 0.620 & 0.011 \\
image\_47.png & 0.670 & 0.710 & 0.008 \\
image\_48.png & 0.570 & 0.640 & 0.009 \\
image\_49.png & 0.630 & 0.590 & 0.008 \\
image\_50.png & 0.570 & 0.560 & 0.008 \\

\midrule
\textbf{Average (COCO, 1--25)}     & 0.591 & 0.683 & 0.007 \\
\textbf{Average (CelebA, 26--50)} & 0.622 & 0.640 & 0.009 \\
\textbf{Average (Overall, 1--50)} & 0.607 & 0.662 & 0.008 \\

\end{longtable}
\endgroup


\begingroup
\small
\setlength{\tabcolsep}{4pt}
\renewcommand{\arraystretch}{0.95}

\begin{longtable}{lccc}
\caption{Non-semantic attack on the \textit{StegaHiDDeN} dataset. Per-image bit accuracy for each decoder: $\mathrm{BA}_{\text{HiDDeN}}$ and $\mathrm{BA}_{\text{Stega}}$, with LPIPS (Similarity Score). Images 1--25: COCO, 26--50: CelebA.}
\label{tab:P3_SH_NS}\\
\toprule
Image & $\mathrm{BA}_{\text{HiDDeN}}$ & $\mathrm{BA}_{\text{Stega}}$ & LPIPS \\
\midrule
\endfirsthead

\toprule
Image & $\mathrm{BA}_{\text{HiDDeN}}$ & $\mathrm{BA}_{\text{Stega}}$ & LPIPS \\
\midrule
\endhead

\midrule
\multicolumn{4}{r}{\textit{Continued on next page}}\\
\endfoot

\bottomrule
\endlastfoot

image\_1.png  & 0.570 & 1.000 & 0.007 \\
image\_2.png  & 0.670 & 0.990 & 0.016 \\
image\_3.png  & 0.600 & 1.000 & 0.008 \\
image\_4.png  & 0.730 & 0.950 & 0.008 \\
image\_5.png  & 0.670 & 0.970 & 0.006 \\
image\_6.png  & 0.600 & 1.000 & 0.007 \\
image\_7.png  & 0.600 & 1.000 & 0.007 \\
image\_8.png  & 0.700 & 1.000 & 0.010 \\
image\_9.png  & 0.670 & 1.000 & 0.012 \\
image\_10.png & 0.700 & 1.000 & 0.009 \\
image\_11.png & 0.600 & 0.990 & 0.010 \\
image\_12.png & 0.570 & 1.000 & 0.009 \\
image\_13.png & 0.670 & 0.980 & 0.008 \\
image\_14.png & 0.600 & 1.000 & 0.008 \\
image\_15.png & 0.670 & 0.990 & 0.011 \\
image\_16.png & 0.670 & 1.000 & 0.008 \\
image\_17.png & 0.630 & 0.950 & 0.009 \\
image\_18.png & 0.600 & 0.990 & 0.009 \\
image\_19.png & 0.700 & 0.990 & 0.013 \\
image\_20.png & 0.700 & 1.000 & 0.011 \\
image\_21.png & 0.670 & 1.000 & 0.008 \\
image\_22.png & 0.570 & 0.990 & 0.008 \\
image\_23.png & 0.700 & 0.930 & 0.008 \\
image\_24.png & 0.570 & 1.000 & 0.008 \\
image\_25.png & 0.570 & 1.000 & 0.009 \\
image\_26.png & 0.570 & 1.000 & 0.011 \\
image\_27.png & 0.630 & 0.980 & 0.010 \\
image\_28.png & 0.530 & 0.990 & 0.007 \\
image\_29.png & 0.830 & 0.970 & 0.008 \\
image\_30.png & 0.630 & 0.980 & 0.009 \\
image\_31.png & 0.700 & 0.990 & 0.012 \\
image\_32.png & 0.730 & 1.000 & 0.011 \\
image\_33.png & 0.600 & 0.980 & 0.010 \\
image\_34.png & 0.670 & 0.990 & 0.008 \\
image\_35.png & 0.730 & 0.990 & 0.011 \\
image\_36.png & 0.730 & 0.990 & 0.007 \\
image\_37.png & 0.670 & 0.950 & 0.014 \\
image\_38.png & 0.570 & 1.000 & 0.011 \\
image\_39.png & 0.670 & 1.000 & 0.006 \\
image\_40.png & 0.670 & 1.000 & 0.011 \\
image\_41.png & 0.730 & 1.000 & 0.006 \\
image\_42.png & 0.700 & 0.990 & 0.010 \\
image\_43.png & 0.630 & 0.990 & 0.010 \\
image\_44.png & 0.770 & 0.980 & 0.010 \\
image\_45.png & 0.770 & 1.000 & 0.007 \\
image\_46.png & 0.670 & 0.990 & 0.010 \\
image\_47.png & 0.730 & 0.950 & 0.008 \\
image\_48.png & 0.700 & 1.000 & 0.017 \\
image\_49.png & 0.730 & 1.000 & 0.006 \\
image\_50.png & 0.570 & 0.980 & 0.011 \\

\midrule
\textbf{Average (COCO, 1--25)}     & 0.640 & 0.989 & 0.009 \\
\textbf{Average (CelebA, 26--50)} & 0.677 & 0.988 & 0.010 \\
\textbf{Average (Overall, 1--50)} & 0.659 & 0.988 & 0.009 \\

\end{longtable}
\endgroup



\begingroup
\small
\setlength{\tabcolsep}{4pt}
\renewcommand{\arraystretch}{0.95}

\begin{longtable}{lccc}
\caption{Semantic attack on the \textit{StegaHiDDeN} dataset \textbf{after} a non-semantic attack (i.e., Non-semantic $\rightarrow$ Semantic). Per-image bit accuracy for each decoder: $\mathrm{BA}_{\text{HiDDeN}}$ and $\mathrm{BA}_{\text{Stega}}$, with LPIPS (Similarity Score). Images 1--25: COCO, 26--50: CelebA.}
\label{tab:P3_SH_NS_S}\\
\toprule
Image & $\mathrm{BA}_{\text{HiDDeN}}$ & $\mathrm{BA}_{\text{Stega}}$ & LPIPS \\
\midrule
\endfirsthead

\toprule
Image & $\mathrm{BA}_{\text{HiDDeN}}$ & $\mathrm{BA}_{\text{Stega}}$ & LPIPS \\
\midrule
\endhead

\midrule
\multicolumn{4}{r}{\textit{Continued on next page}}\\
\endfoot

\bottomrule
\endlastfoot

image\_1.png  & 0.600 & 0.570 & 0.151 \\
image\_2.png  & 0.600 & 0.630 & 0.198 \\
image\_3.png  & 0.600 & 0.620 & 0.132 \\
image\_4.png  & 0.670 & 0.630 & 0.155 \\
image\_5.png  & 0.670 & 0.610 & 0.119 \\
image\_6.png  & 0.570 & 0.610 & 0.171 \\
image\_7.png  & 0.570 & 0.620 & 0.150 \\
image\_8.png  & 0.630 & 0.670 & 0.160 \\
image\_9.png  & 0.630 & 0.630 & 0.205 \\
image\_10.png & 0.630 & 0.580 & 0.168 \\
image\_11.png & 0.530 & 0.680 & 0.142 \\
image\_12.png & 0.530 & 0.630 & 0.155 \\
image\_13.png & 0.570 & 0.660 & 0.144 \\
image\_14.png & 0.630 & 0.690 & 0.131 \\
image\_15.png & 0.670 & 0.640 & 0.181 \\
image\_16.png & 0.670 & 0.710 & 0.171 \\
image\_17.png & 0.630 & 0.580 & 0.123 \\
image\_18.png & 0.500 & 0.560 & 0.134 \\
image\_19.png & 0.630 & 0.570 & 0.166 \\
image\_20.png & 0.630 & 0.580 & 0.195 \\
image\_21.png & 0.570 & 0.700 & 0.175 \\
image\_22.png & 0.570 & 0.570 & 0.131 \\
image\_23.png & 0.570 & 0.580 & 0.153 \\
image\_24.png & 0.630 & 0.580 & 0.120 \\
image\_25.png & 0.570 & 0.580 & 0.149 \\
image\_26.png & 0.570 & 0.580 & 0.175 \\
image\_27.png & 0.570 & 0.570 & 0.129 \\
image\_28.png & 0.600 & 0.580 & 0.110 \\
image\_29.png & 0.800 & 0.580 & 0.130 \\
image\_30.png & 0.630 & 0.690 & 0.144 \\
image\_31.png & 0.600 & 0.550 & 0.115 \\
image\_32.png & 0.730 & 0.570 & 0.116 \\
image\_33.png & 0.600 & 0.580 & 0.134 \\
image\_34.png & 0.470 & 0.650 & 0.195 \\
image\_35.png & 0.630 & 0.570 & 0.113 \\
image\_36.png & 0.670 & 0.580 & 0.114 \\
image\_37.png & 0.630 & 0.650 & 0.187 \\
image\_38.png & 0.530 & 0.660 & 0.167 \\
image\_39.png & 0.630 & 0.860 & 0.090 \\
image\_40.png & 0.570 & 0.530 & 0.161 \\
image\_41.png & 0.770 & 0.700 & 0.108 \\
image\_42.png & 0.530 & 0.590 & 0.176 \\
image\_43.png & 0.670 & 0.650 & 0.159 \\
image\_44.png & 0.630 & 0.720 & 0.168 \\
image\_45.png & 0.700 & 0.570 & 0.106 \\
image\_46.png & 0.670 & 0.580 & 0.101 \\
image\_47.png & 0.730 & 0.620 & 0.133 \\
image\_48.png & 0.630 & 0.570 & 0.200 \\
image\_49.png & 0.570 & 0.610 & 0.141 \\
image\_50.png & 0.570 & 0.550 & 0.124 \\

\midrule
\textbf{Average (COCO, 1--25)}     & 0.603 & 0.619 & 0.155 \\
\textbf{Average (CelebA, 26--50)} & 0.628 & 0.614 & 0.140 \\
\textbf{Average (Overall, 1--50)} & 0.615 & 0.617 & 0.148 \\

\end{longtable}
\endgroup

\begingroup
\small
\setlength{\tabcolsep}{4pt}
\renewcommand{\arraystretch}{0.95}

\begin{longtable}{lccc}
\caption{Semantic attack on the \textit{StegaHiDDeN} dataset. Per-image bit accuracy for each decoder: $\mathrm{BA}_{\text{HiDDeN}}$ and $\mathrm{BA}_{\text{Stega}}$, with LPIPS (Similarity Score). Images 1--25: COCO, 26--50: CelebA.}
\label{tab:P3_SH_S}\\
\toprule
Image & $\mathrm{BA}_{\text{HiDDeN}}$ & $\mathrm{BA}_{\text{Stega}}$ & LPIPS \\
\midrule
\endfirsthead

\toprule
Image & $\mathrm{BA}_{\text{HiDDeN}}$ & $\mathrm{BA}_{\text{Stega}}$ & LPIPS \\
\midrule
\endhead

\midrule
\multicolumn{4}{r}{\textit{Continued on next page}}\\
\endfoot

\bottomrule
\endlastfoot

image\_1.png & 0.900 & 0.580 & 0.127 \\
image\_2.png & 0.830 & 0.580 & 0.199 \\
image\_3.png & 0.900 & 0.580 & 0.100 \\
image\_4.png & 0.830 & 0.570 & 0.162 \\
image\_5.png & 0.900 & 0.580 & 0.117 \\
image\_6.png & 0.930 & 0.570 & 0.131 \\
image\_7.png & 0.830 & 0.570 & 0.141 \\
image\_8.png & 0.770 & 0.660 & 0.180 \\
image\_9.png & 0.930 & 0.570 & 0.145 \\
image\_10.png & 0.730 & 0.600 & 0.214 \\
image\_11.png & 0.900 & 0.580 & 0.123 \\
image\_12.png & 0.930 & 0.580 & 0.124 \\
image\_13.png & 0.930 & 0.580 & 0.132 \\
image\_14.png & 0.830 & 0.580 & 0.128 \\
image\_15.png & 0.730 & 0.600 & 0.183 \\
image\_16.png & 0.930 & 0.580 & 0.120 \\
image\_17.png & 1.000 & 0.580 & 0.118 \\
image\_18.png & 0.970 & 0.550 & 0.119 \\
image\_19.png & 0.900 & 0.570 & 0.157 \\
image\_20.png & 0.800 & 0.580 & 0.191 \\
image\_21.png & 0.830 & 0.580 & 0.136 \\
image\_22.png & 0.970 & 0.580 & 0.147 \\
image\_23.png & 0.870 & 0.570 & 0.167 \\
image\_24.png & 0.930 & 0.580 & 0.119 \\
image\_25.png & 0.930 & 0.580 & 0.130 \\
image\_26.png & 0.930 & 0.580 & 0.146 \\
image\_27.png & 0.930 & 0.580 & 0.125 \\
image\_28.png & 0.870 & 0.580 & 0.099 \\
image\_29.png & 0.970 & 0.580 & 0.141 \\
image\_30.png & 0.930 & 0.570 & 0.102 \\
image\_31.png & 0.970 & 0.540 & 0.116 \\
image\_32.png & 0.900 & 0.580 & 0.137 \\
image\_33.png & 0.970 & 0.580 & 0.143 \\
image\_34.png & 0.730 & 0.700 & 0.242 \\
image\_35.png & 0.930 & 0.570 & 0.135 \\
image\_36.png & 0.970 & 0.580 & 0.127 \\
image\_37.png & 1.000 & 0.560 & 0.122 \\
image\_38.png & 0.730 & 0.570 & 0.170 \\
image\_39.png & 0.800 & 0.620 & 0.112 \\
image\_40.png & 0.830 & 0.580 & 0.150 \\
image\_41.png & 0.970 & 0.580 & 0.080 \\
image\_42.png & 0.930 & 0.550 & 0.124 \\
image\_43.png & 0.970 & 0.560 & 0.089 \\
image\_44.png & 0.930 & 0.580 & 0.104 \\
image\_45.png & 0.930 & 0.580 & 0.086 \\
image\_46.png & 0.970 & 0.580 & 0.114 \\
image\_47.png & 0.930 & 0.570 & 0.115 \\
image\_48.png & 0.870 & 0.570 & 0.195 \\
image\_49.png & 0.930 & 0.580 & 0.104 \\
image\_50.png & 0.970 & 0.580 & 0.110 \\

\midrule
\textbf{Average (COCO, 1--25)}     & 0.880 & 0.581 & 0.144 \\
\textbf{Average (CelebA, 26--50)} & 0.914 & 0.580 & 0.128 \\
\textbf{Average (Overall, 1--50)} & 0.897 & 0.581 & 0.136 \\

\end{longtable}
\endgroup


\begingroup
\small
\setlength{\tabcolsep}{4pt}
\renewcommand{\arraystretch}{0.95}

\begin{longtable}{lccc}
\caption{Non-semantic attack on the \textit{StegaHiDDeN} dataset \textbf{after} a Semantic attack (i.e., Semantic $\rightarrow$ Non-semantic). Per-image bit accuracy for each decoder: $\mathrm{BA}_{\text{HiDDeN}}$ and $\mathrm{BA}_{\text{Stega}}$, with LPIPS (Similarity Score). Images 1--25: COCO, 26--50: CelebA.}
\label{tab:P3_SH_S_NS}\\
\toprule
Image & $\mathrm{BA}_{\text{HiDDeN}}$ & $\mathrm{BA}_{\text{Stega}}$ & LPIPS \\
\midrule
\endfirsthead

\toprule
Image & $\mathrm{BA}_{\text{HiDDeN}}$ & $\mathrm{BA}_{\text{Stega}}$ & LPIPS \\
\midrule
\endhead

\midrule
\multicolumn{4}{r}{\textit{Continued on next page}}\\
\endfoot

\bottomrule
\endlastfoot

image\_1.png  & 0.570 & 0.550 & 0.007 \\
image\_2.png  & 0.630 & 0.590 & 0.011 \\
image\_3.png  & 0.570 & 0.540 & 0.008 \\
image\_4.png  & 0.670 & 0.580 & 0.007 \\
image\_5.png  & 0.670 & 0.610 & 0.006 \\
image\_6.png  & 0.570 & 0.550 & 0.008 \\
image\_7.png  & 0.670 & 0.610 & 0.007 \\
image\_8.png  & 0.630 & 0.720 & 0.008 \\
image\_9.png  & 0.600 & 0.560 & 0.011 \\
image\_10.png & 0.600 & 0.600 & 0.008 \\
image\_11.png & 0.600 & 0.620 & 0.009 \\
image\_12.png & 0.600 & 0.650 & 0.009 \\
image\_13.png & 0.570 & 0.610 & 0.009 \\
image\_14.png & 0.570 & 0.620 & 0.007 \\
image\_15.png & 0.630 & 0.590 & 0.009 \\
image\_16.png & 0.570 & 0.540 & 0.008 \\
image\_17.png & 0.600 & 0.530 & 0.011 \\
image\_18.png & 0.530 & 0.590 & 0.009 \\
image\_19.png & 0.630 & 0.570 & 0.013 \\
image\_20.png & 0.570 & 0.590 & 0.008 \\
image\_21.png & 0.530 & 0.580 & 0.009 \\
image\_22.png & 0.630 & 0.640 & 0.008 \\
image\_23.png & 0.600 & 0.580 & 0.007 \\
image\_24.png & 0.630 & 0.610 & 0.009 \\
image\_25.png & 0.600 & 0.610 & 0.010 \\
image\_26.png & 0.600 & 0.530 & 0.013 \\
image\_27.png & 0.530 & 0.600 & 0.010 \\
image\_28.png & 0.570 & 0.590 & 0.008 \\
image\_29.png & 0.800 & 0.620 & 0.008 \\
image\_30.png & 0.630 & 0.560 & 0.009 \\
image\_31.png & 0.570 & 0.580 & 0.015 \\
image\_32.png & 0.500 & 0.600 & 0.010 \\
image\_33.png & 0.630 & 0.550 & 0.011 \\
image\_34.png & 0.530 & 0.670 & 0.008 \\
image\_35.png & 0.700 & 0.590 & 0.012 \\
image\_36.png & 0.670 & 0.580 & 0.007 \\
image\_37.png & 0.570 & 0.610 & 0.014 \\
image\_38.png & 0.500 & 0.560 & 0.008 \\
image\_39.png & 0.630 & 0.630 & 0.005 \\
image\_40.png & 0.570 & 0.630 & 0.012 \\
image\_41.png & 0.770 & 0.600 & 0.007 \\
image\_42.png & 0.630 & 0.550 & 0.012 \\
image\_43.png & 0.700 & 0.600 & 0.010 \\
image\_44.png & 0.700 & 0.560 & 0.011 \\
image\_45.png & 0.730 & 0.620 & 0.007 \\
image\_46.png & 0.670 & 0.630 & 0.011 \\
image\_47.png & 0.630 & 0.630 & 0.009 \\
image\_48.png & 0.600 & 0.610 & 0.017 \\
image\_49.png & 0.570 & 0.620 & 0.007 \\
image\_50.png & 0.530 & 0.560 & 0.013 \\

\midrule
\textbf{Average (COCO, 1--25)}     & 0.602 & 0.594 & 0.009 \\
\textbf{Average (CelebA, 26--50)} & 0.621 & 0.595 & 0.010 \\
\textbf{Average (Overall, 1--50)} & 0.611 & 0.594 & 0.009 \\

\end{longtable}
\endgroup
